# Supplementary material for: Photoelectron spectroscopy investigation of the temperature-induced deprotonation and substrate-mediated hydrogen transfer in a hydroxyphenyl-substituted porphyrin
Source: arXiv:1502.07185 ancillary file (2015-02-25)
Supplement: Supplementary file 1 [file Supplemental_Information.pdf]

# Supplemental Information for

## Photoelectron spectroscopy investigation of the temperature-induced deprotonation and substrate-mediated hydrogen transfer of a hydroxyphenyl-substituted porphyrin

Lars Smykalla[a], Pavel Shukrynau[a], Carola Mende[b], Heinrich Lang[b], Martin Knupfer[c], Michael Hietschold[a]

[a] *Technische Universität Chemnitz, Institute of Physics, Solid Surfaces Analysis Group, 09107 Chemnitz, Germany*
[b] *Technische Universität Chemnitz, Institute of Chemistry, Inorganic Chemistry, 09107 Chemnitz, Germany*
[c] *Electronic and Optical Properties Department, IFW Dresden, D-01171 Dresden, Germany*

---

### Scanning tunneling microscopy of the $H_2$THPP layer after annealing to 400 °C

5,10,15,20-tetra(*p*-hydroxyphenyl)porphyrin ($H_2$THPP) molecules were deposited on a clean Au(111) surface by organic molecular beam epitaxy in UHV. Scanning tunneling microscopy (STM) was measured with a VT-STM from Omicron at room temperature. The sample was subsequently heated to a temperature of $\approx$ 400 °C. STM images showed that in many areas the self-assembled structures were destroyed and the arrangement of the molecules became disordered as shown in Fig. S1. At submonolayer coverage, it is clearly seen that the molecules partially decomposed which hinders an identification of the individual molecules. Dendritic oligomer-like agglomerations are formed which can only be moved by the STM tip as whole as demonstrated in Fig. S1(a),(b) (the blue arrows mark the same vacancy which shows the rotation by tip manipulation.) This shows that these molecules are covalently linked by dehydrogenative intermolecular C–C coupling.

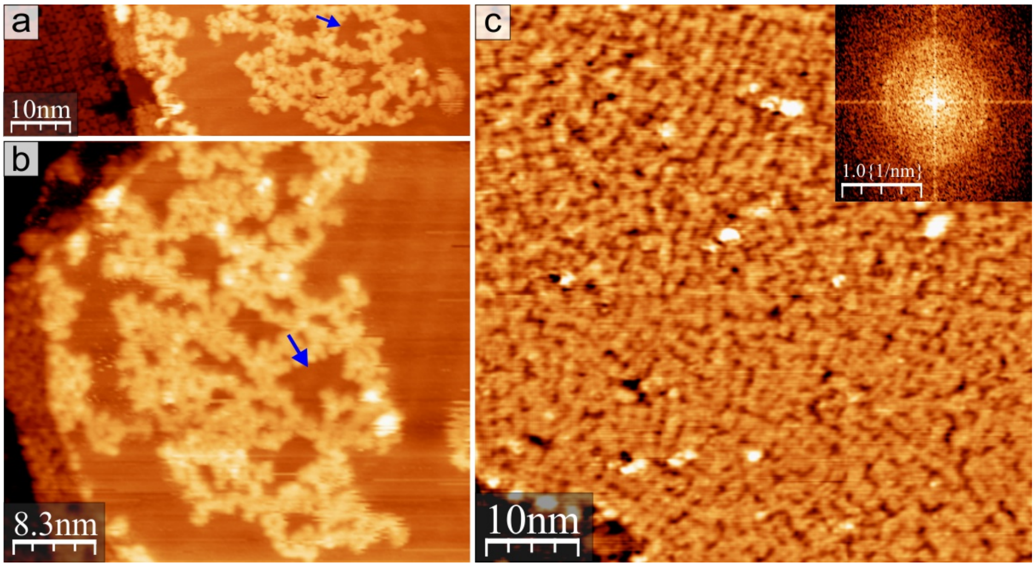


Figure S1: STM images of $H_2$THPP molecules on Au(111) after annealing to 400 °C: (a), (b) submonolayer coverage – partially decomposition and formation of dendritic oligomer-like arrangement due to intermolecular C–C coupling. (c) coverage of a full monolayer – the molecular arrangement became disordered in most areas. Inset: The Fourier-transformation of the image shows disorder in the molecular layer.

## Carbon 1s core level spectra of $H_2$THPP on Ag(110)

The C 1s core level spectra of $H_2$THPP on Ag(110) are shown in Fig. S2. The change of the peak shape with increasing temperature is similar as for $H_2$THPP on Au(111) which is discussed in the main text. After annealing of the layer at 300 °C, the signal changes due to starting decomposition and coupling of the molecules, which is more pronounced on Ag(110) than on Au(111) after 300 °C. Annealing at 300 °C for 5 min was not enough to completely desorb the molecular multilayer, which is indicated by the small decrease of the C 1s signal and the absence of the typical multilayer → monolayer shift of the signal to lower binding energy (as well as the attenuation of the Ag 3d peaks and the not visible Fermi edge).

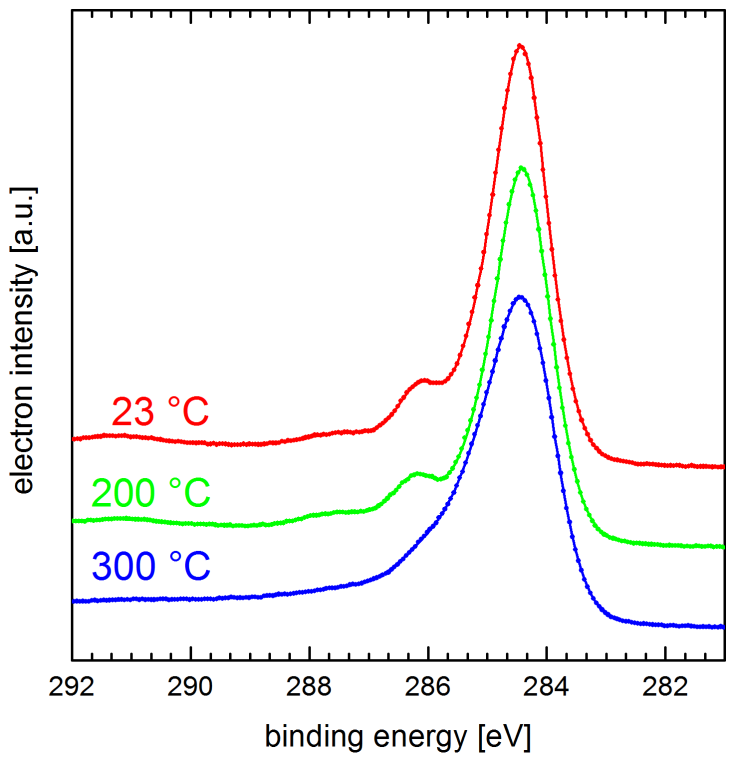


Figure S2: Evolution of the C 1s core level spectra of $H_2$THPP on Ag(110) with increasing annealing temperature. The excitation photon energy was $E_{\text{exc}} = 390\,\text{eV}$).

## Comparison of the valence band spectra with Density Functional Theory calculations

Calculations were performed with the Grid-based Projector Augmented Wave method (GPAW). Molecules were placed in a large box of vacuum with zero boundary conditions and fully relaxed. Computational resources were provided by the "Chemnitzer Hochleistungs-Linux-Cluster" (CHiC) at the Technische Universität Chemnitz. Figure S3 shows the density of states calculated with DFT in comparison with the background-corrected photoelectron valance band spectrum. It was found that the spectral shape can be nicely reproduced with a Gaussian broadening of the molecular states of 0.4 eV. However, this is not the case for the exact energetic positions. For vdW-F2, the well known underestimation of the HOMO–LUMO gap of the generalized gradient approximation becomes obvious. Whereas, for Becke's three parameter hybrid-DFT functional (B3LYP) all states are now moved too far away from $E_F$ compared to the valance band spectra of the $H_2$THPP multilayer, due to the too large amount of exact exchange in B3LYP. Furthermore, with the help of DFT it becomes clear that the peak discussed in the main text at 1.5 eV binding energy is a convolution of the HOMO and HOMO−1.

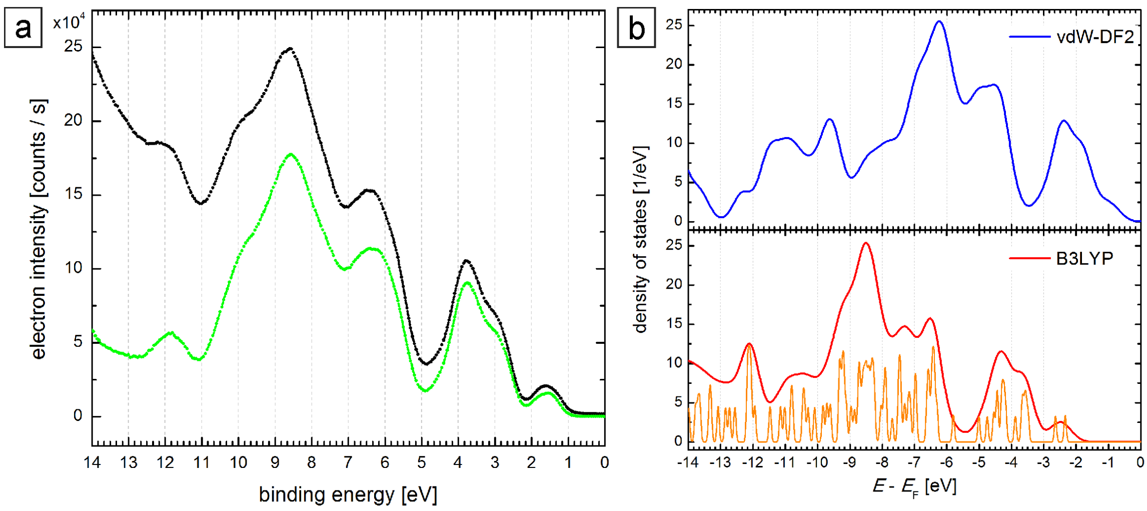


Figure S3: (a) Valence band spectra of a ≈ 2.4 nm thick layer of $H_2$THPP ($E_{exc}$ = 22 eV). Measured data is in black and background corrected valence band in green. (b) Calculated density of states of $H_2$THPP in gas-phase for the vdW-DF2 (top) and the hybrid-DFT B3LYP (bottom) xc-functionals (blue/red 0.4 eV, orange 0.02 eV broadening).
